# Supplementary material for: CGOF++: Controllable 3D Face Synthesis with Conditional Generative Occupancy Fields
Source: arXiv:2211.13251 source file (2023-10-29)
Supplement: Supplementary file 1 [file supmat_main.tex]

\section{Implementation Details}
\paragraph{Network Architectures.}
This project is based on the released code of \piganc and Deep3DFaceRecon~\cite{deng2019accurate}. We use the same architectures for the generator and discriminator, as well as the main training process in from the \pigan. To implement our proposed conditional Generative Occupancy Field (cGOF), we integrate a deep 3D face reconstruction model \dfrc to reconstruct 3DMM parameters from the generated images for the 3DMM reconstruction parameter loss $\mathcal{L}_\text{recon}$.

\paragraph{\label{coor_align}Coordinate System Alignment.}
We align the 3DMM meshes to \pigan in order to impose the 3D losses.
We first use the pretrained \pigan to generate multi-view images of various face instances in the canonical viewpoint and use the \dfr to reconstruct 3DMM meshes $M$ for the generated faces, on which we define a set of landmark $\mathbf{l}_\text{3D}$.
Let $K_\text{recon}$ and $E_\text{recon}$ be the intrinsic and extrinsic matrices for 3DMM, and $K_\text{pigan}$ and $E_\text{pigan}$ the counterparts for \pigan respectively.
Let $T_\text{R2P}$ be the transformation matrix from 3DMM to \pigan that we would like to estimate.
We directly optimize this transformation matrix by minimizing the difference of 2D projections of a set of landmarks obtained from the original mesh $M$ and the transformed mesh $M' = T_\text{R2P} \cdot M$, denoted as $\mathbf{l}_\text{2D}$ and $\mathbf{l}'_\text{2D}$:
\begin{equation}
\begin{aligned}
\label{eqn:coor_align}
T_\text{R2P}^* &= \argmin_{T_\text{R2P}} \| \mathbf{l}_\text{2D} - \mathbf{l}'_\text{2D} \|_1, \\
\text{where} \quad
\mathbf{l}_\text{2D} &= K_\text{recon} \cdot E_\text{recon} \cdot \mathbf{l}_\text{3D}, \\
\mathbf{l}'_\text{2D} &= K_\text{pigan} \cdot E_\text{pigan} \cdot T_\text{R2P} \cdot \mathbf{l}_\text{3D}.
\end{aligned}
\end{equation}

\paragraph{Background Modeling.}
We model the background by setting the weight of the last sample point along each ray to be $w_N = 1- \sum_{i=1}^{N-1}{w_i}$, where $w_i = T_i \cdot (1-\expo{-\absrp_i \deltatime_i})$ is weight of the rest of the sample points along the ray, including both the mesh-guided samples and the volume samples.

\paragraph{Hyper-Parameters and Volume Sampling.}
\cref{supmat:tab:param_set} summarizes all hyper-parameters.
We sample $12$ coarse points evenly in the volume to and obtain $N_\text{vol}=12$ fine points as introduced in~\cite{mildenhall2020nerf}.
Only $N_\text{vol} = 12$ fine points and the $N_\text{surf} = 12$ points sampled around the 3DMM input mesh are used for rendering and optimization with gradient backpropagation.
The final model is trained for 72 hours on 8 GeForce GTX TITAN X GPUs.

\section{Additional Qualitative Results}
\subsection{Additional Results with Pose Variations}
We present large pose results for \ganctrlc in \cref{Fig:poses_gancontrol}, \discoc in \cref{Fig:poses_disco}, \headnerfc in \cref{Fig:poses_headnerf} and \piganc in \cref{Fig:poses_pigan}.
Previous methods fail to generate plausible face image when the camera pose gets larger (\eg $> 60^\circ$), including NeRF-based methods (\headnerf and \pigan).
Nevertheless, as shown in \cref{Fig:poses_cgof}, our method produces plausible \emph{3D consistent} face images even in extremely large poses.
Note that, to get rid the view-dependent affect, we follow~\cite{gu2022stylenerf, hong2021headnerf} and remove the dependence of the radiance colors on the viewing direction by setting the view direction to a constant $(0,0,-1)$ when evaluating the radiance colors of the sample points.

\subsection{Additional Results with Expression Variations}
We present more results on the expression control, comparing our method against two state-of-the-art controllable face synthesis methods, one attribute-guided \ganctrlc and the other 3DMM-guided \discoc.
\cref{Fig:exps_gancontrol,Fig:exps_disco,Fig:exps_cgof} show the generated faces using \ganctrl, \disco and our method respectively.
For each figure, the first column shows a reference image, columns 2 to 5 show images generated with mild expressions, and columns 6 to 9 show images generated with wilder expressions.
Each row corresponds to the same person, and each column corresponds to the same expression.

\input{supmat/tabs/hyper_param}

In \cref{Fig:exps_gancontrol}, we can see that \ganctrl fails to preserve the identity as well as other factors of the face image (\eg background), when changing only the facial expression code.
A few examples are highlighted in red.
Moreover, we observe that with the original range of the expression parameters, the model results in only a small variation of expressions, whereas with increased perturbations, it leads to much more significant shape and identity inconsistencies.
We also notice the ``smiling'' attribute tends to strongly correlate with the ``female'' and ``long-hair'' attributes.

In \cref{Fig:exps_disco}, we can see that the \disco fails to impose consistent expression control over the faces.
The blue boxes highlight a few examples, where the same expression code produces different expressions in different faces.
Moreover, the images generated with wild expressions may appear unnatural, such as `exp 5' in \cref{Fig:exps_disco}.

In \cref{Fig:exps_cgof}, we show that our model generates compelling photo-realistic face images with highly consistent, precise expression control.
In each row, only expressions change while other properties remain unchanged, such as identity (shape and texture), hair and background.
In each column, all instances follow the same expression.

In addition, in \cref{Fig:exps_ood_cgof}, we present examples of images generated by our model with \emph{out-of-distribution} expressions, such as frowning, pouting, curling lips, smirking \etc.
Despite that images with such expressions hardly exist in the training data, our model is still able to generate highly plausible images.

\newpage

\begin{figure*}[t!]
    \centering
    \resizebox{1.0\linewidth}{!}{
    \begin{subfigure}[b]{1.0\linewidth}
        \includegraphics[width=\linewidth]{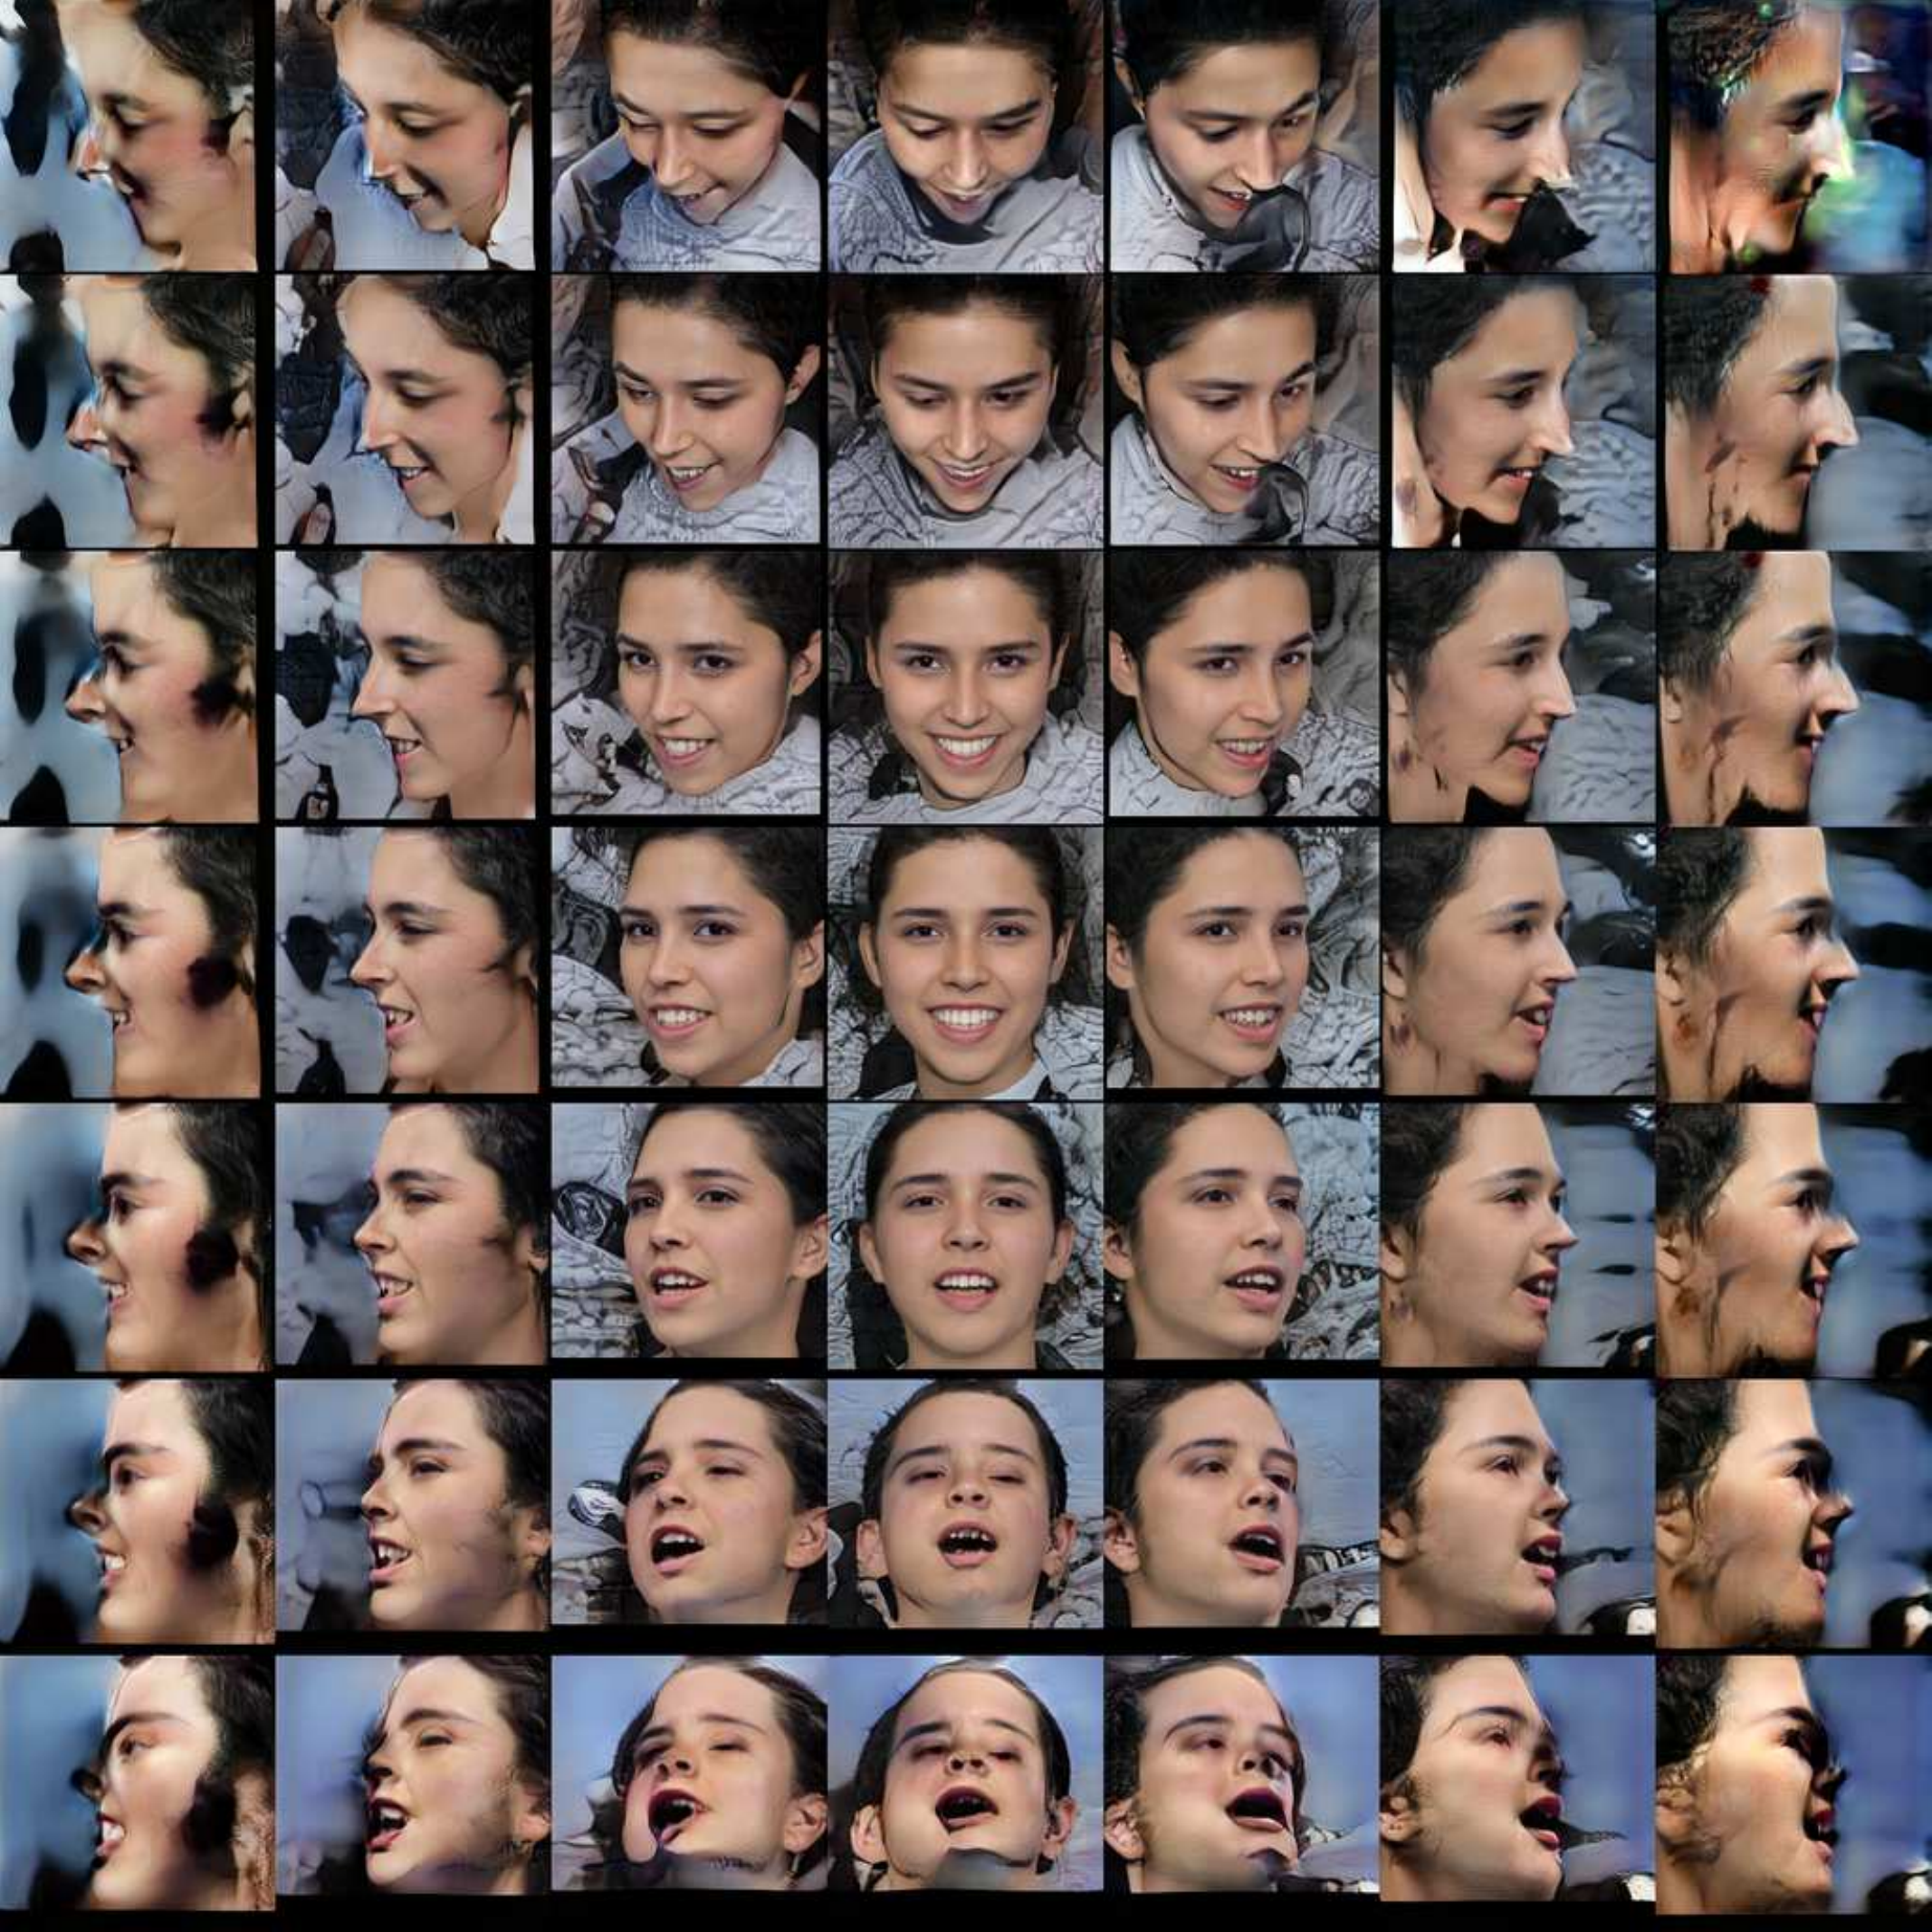}
    \end{subfigure}
    \begin{subfigure}[b]{1.0\linewidth}
        \includegraphics[width=\linewidth]{supmat/figs/poses/gancontrol/g_1_1024.pdf}
    \end{subfigure}
    }
    \resizebox{1.0\linewidth}{!}{
    \begin{subfigure}[b]{1.0\linewidth}
        \includegraphics[width=\linewidth]{supmat/figs/poses/gancontrol/g_2_1024.pdf}
    \end{subfigure}
    \begin{subfigure}[b]{1.0\linewidth}
        \includegraphics[width=\linewidth]{supmat/figs/poses/gancontrol/g_3_1024.pdf}
    \end{subfigure}
    }
    \resizebox{1.0\linewidth}{!}{
    \begin{subfigure}[b]{1.0\linewidth}
        \includegraphics[width=\linewidth]{supmat/figs/poses/gancontrol/g_4_1024.pdf}
    \end{subfigure}
    \begin{subfigure}[b]{1.0\linewidth}
        \includegraphics[width=\linewidth]{supmat/figs/poses/gancontrol/g_5_1024.pdf}
    \end{subfigure}
    }
    \caption{Images generated by GAN-Control~\cite{shoshan2021gancontrol} with different \emph{poses}.}
    \label{Fig:poses_gancontrol}
\end{figure*}

\newpage

\begin{figure*}[t!]
    \centering
    \resizebox{1.0\linewidth}{!}{
    \begin{subfigure}[b]{1.0\linewidth}
        \includegraphics[width=\linewidth]{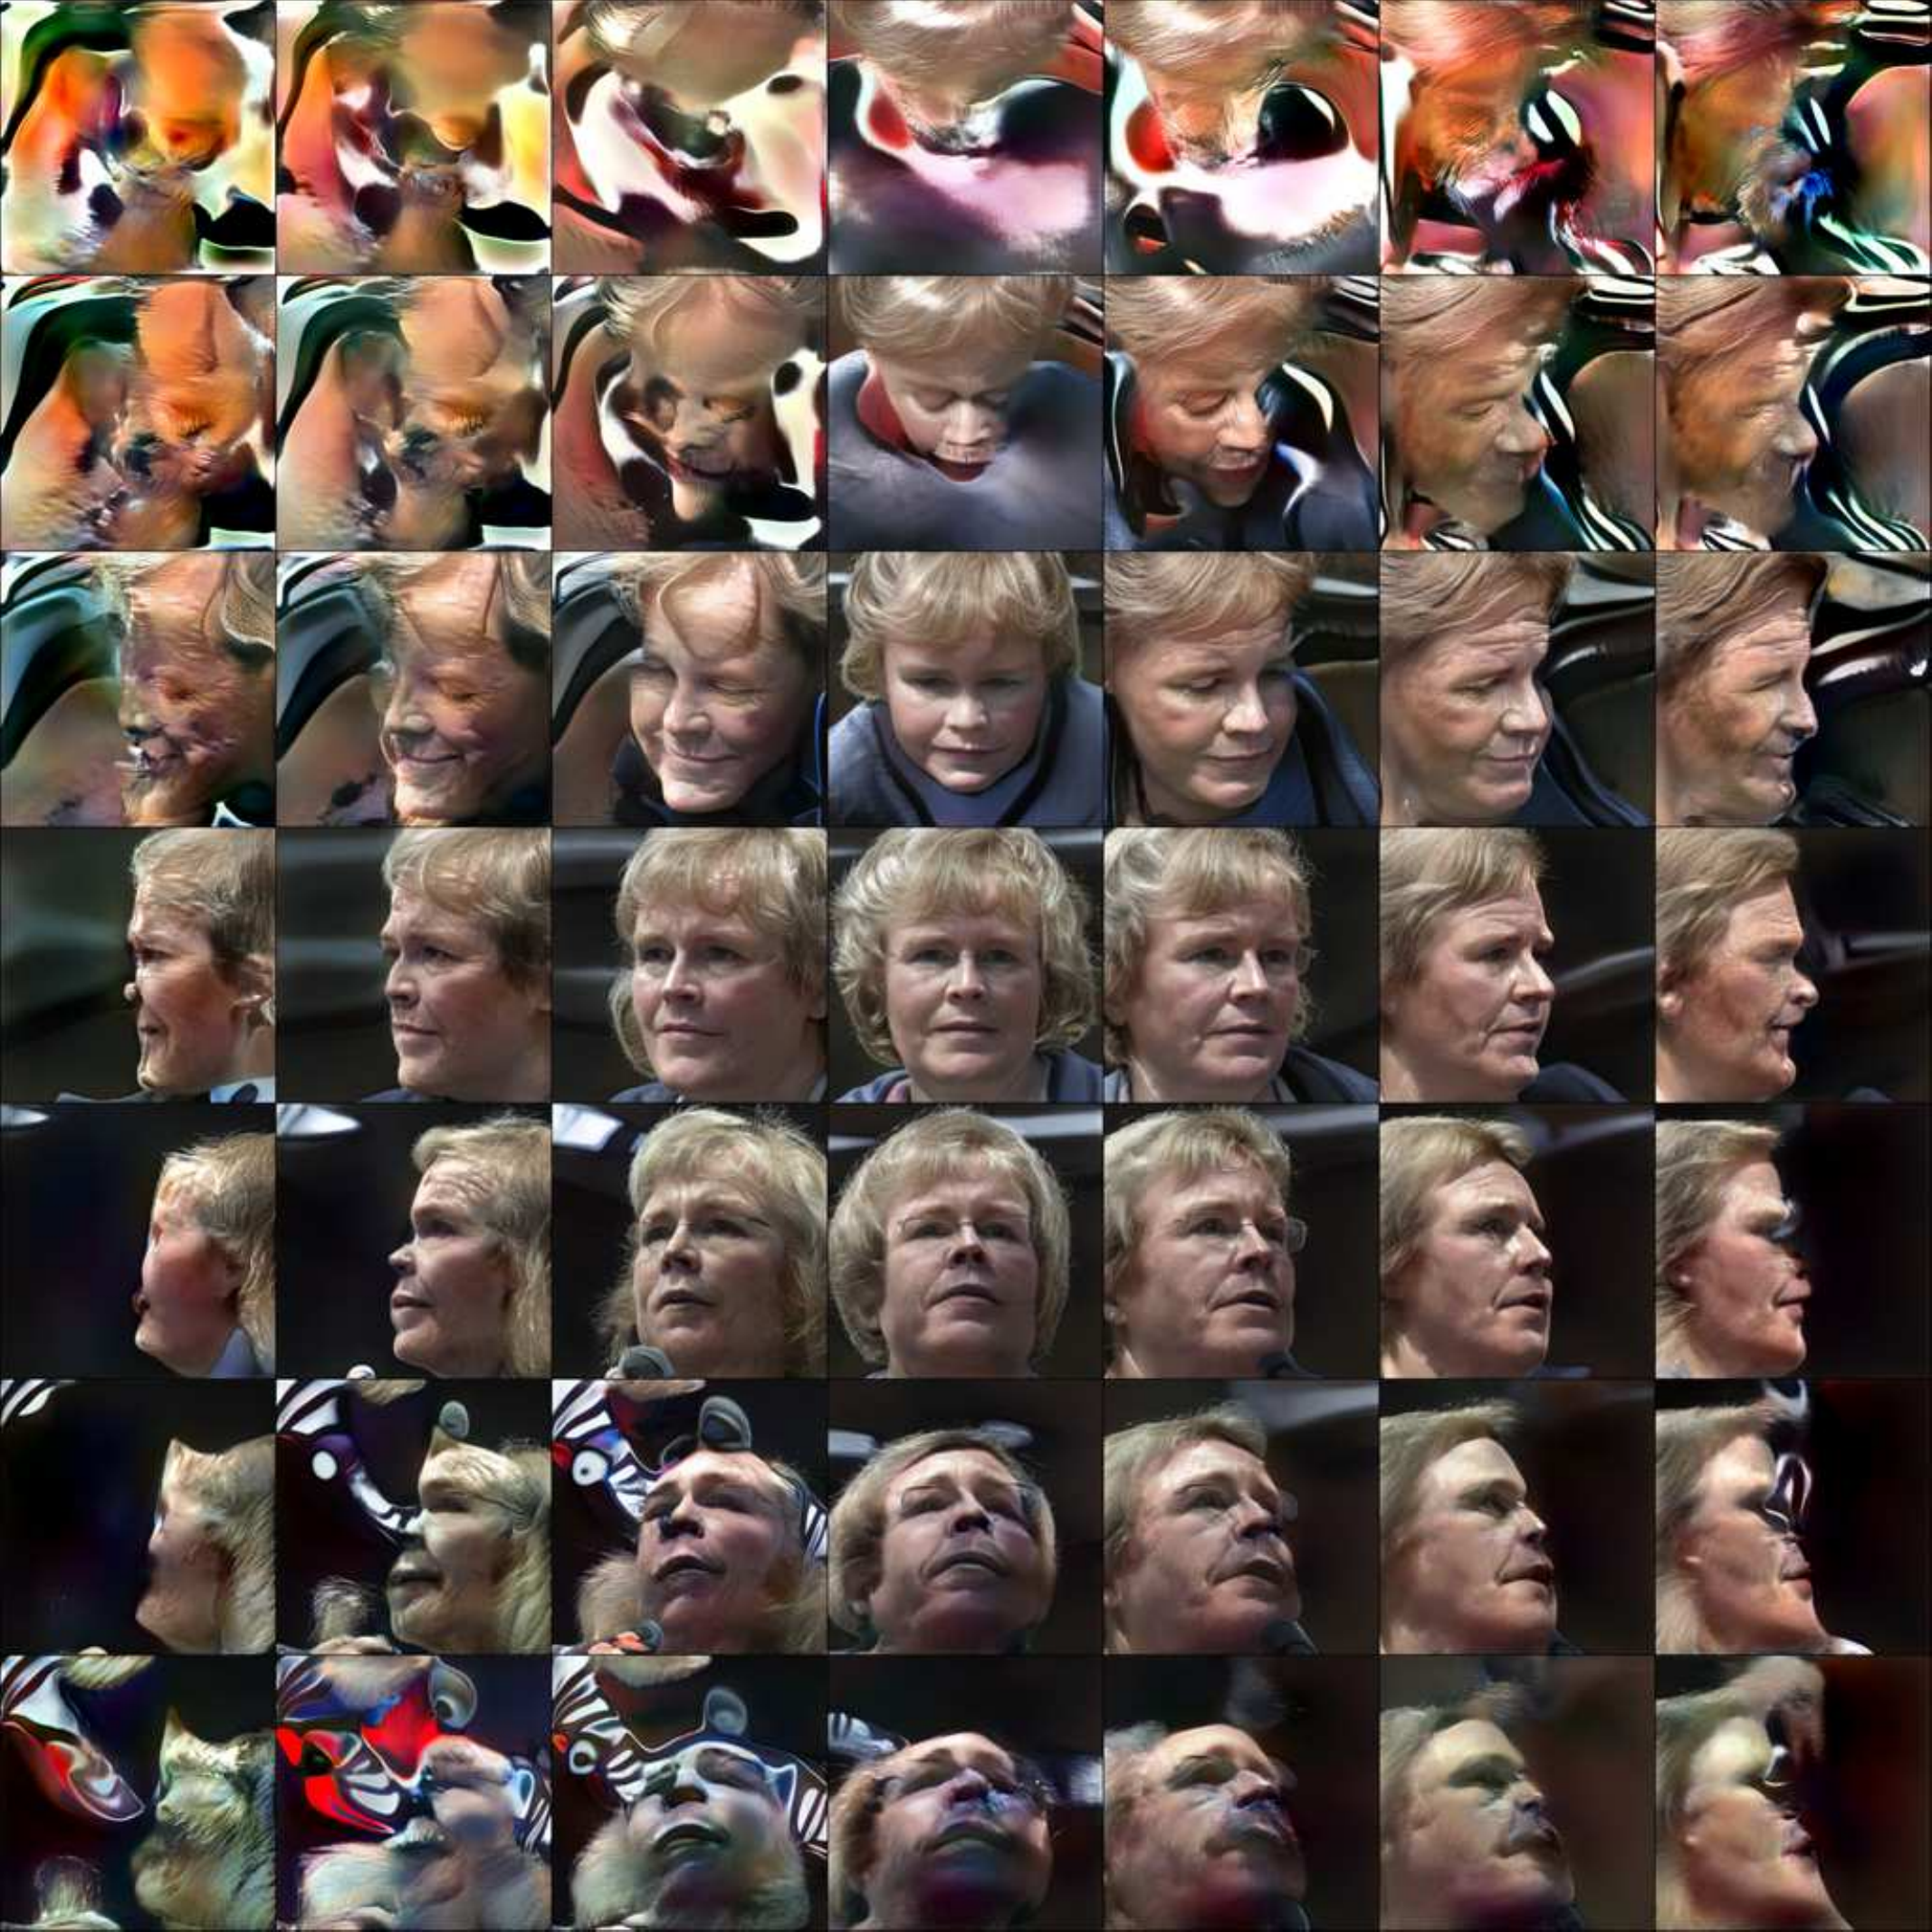}
    \end{subfigure}
    \begin{subfigure}[b]{1.0\linewidth}
        \includegraphics[width=\linewidth]{supmat/figs/poses/disco/d_1_1024.pdf}
    \end{subfigure}
    }
    \resizebox{1.0\linewidth}{!}{
    \begin{subfigure}[b]{1.0\linewidth}
        \includegraphics[width=\linewidth]{supmat/figs/poses/disco/d_2_1024.pdf}
    \end{subfigure}
    \begin{subfigure}[b]{1.0\linewidth}
        \includegraphics[width=\linewidth]{supmat/figs/poses/disco/d_3_1024.pdf}
    \end{subfigure}
    }
    \resizebox{1.0\linewidth}{!}{
    \begin{subfigure}[b]{1.0\linewidth}
        \includegraphics[width=\linewidth]{supmat/figs/poses/disco/d_4_1024.pdf}
    \end{subfigure}
    \begin{subfigure}[b]{1.0\linewidth}
        \includegraphics[width=\linewidth]{supmat/figs/poses/disco/d_5_1024.pdf}
    \end{subfigure}
    }
    \caption{Images generated by DiscoFaceGAN~\cite{deng2020disentangled} with different \emph{poses}.}
    \label{Fig:poses_disco}
\end{figure*}

\newpage

\begin{figure*}[t!]
    \centering
    \resizebox{1.0\linewidth}{!}{
    \begin{subfigure}[b]{1.0\linewidth}
        \includegraphics[width=\linewidth]{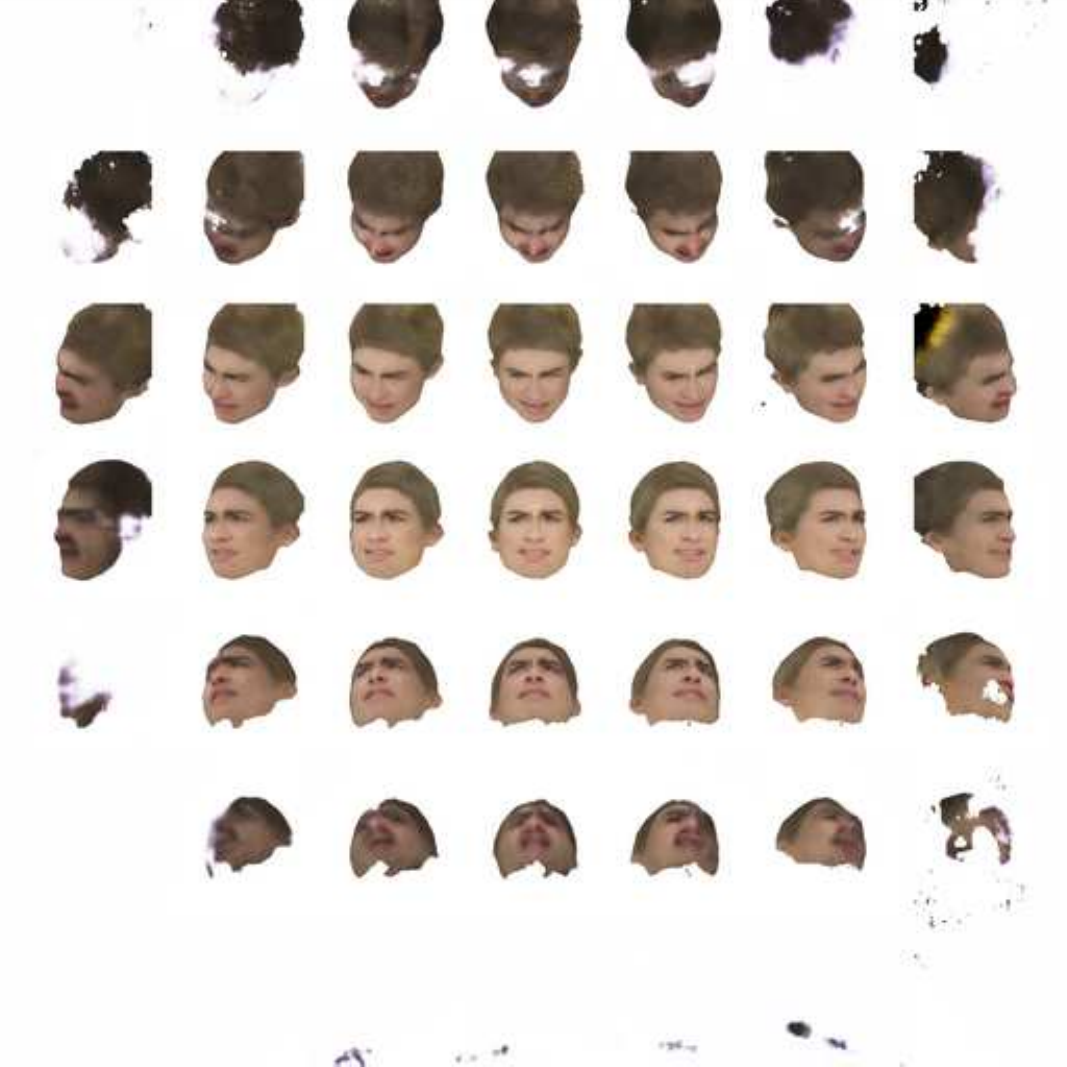}
    \end{subfigure}
    \begin{subfigure}[b]{1.0\linewidth}
        \includegraphics[width=\linewidth]{supmat/figs/poses/headnerf/h_1.pdf}
    \end{subfigure}
    }
    \resizebox{1.0\linewidth}{!}{
    \begin{subfigure}[b]{1.0\linewidth}
        \includegraphics[width=\linewidth]{supmat/figs/poses/headnerf/h_2.pdf}
    \end{subfigure}
    \begin{subfigure}[b]{1.0\linewidth}
        \includegraphics[width=\linewidth]{supmat/figs/poses/headnerf/h_3.pdf}
    \end{subfigure}
    }
    \resizebox{1.0\linewidth}{!}{
    \begin{subfigure}[b]{1.0\linewidth}
        \includegraphics[width=\linewidth]{supmat/figs/poses/headnerf/h_4.pdf}
    \end{subfigure}
    \begin{subfigure}[b]{1.0\linewidth}
        \includegraphics[width=\linewidth]{supmat/figs/poses/headnerf/h_5.pdf}
    \end{subfigure}
    }
    \caption{
    Images generated by HeadNeRF~\cite{hong2021headnerf} with different \emph{poses}.}
    \label{Fig:poses_headnerf}
\end{figure*}

\newpage

\begin{figure*}[t!]
    \centering
    \resizebox{1.0\linewidth}{!}{
    \begin{subfigure}[b]{1.0\linewidth}
        \includegraphics[width=\linewidth]{supmat/figs/poses/pigan/p_0.pdf}
    \end{subfigure}
    \begin{subfigure}[b]{1.0\linewidth}
        \includegraphics[width=\linewidth]{supmat/figs/poses/pigan/p_1.pdf}
    \end{subfigure}
    }
    \resizebox{1.0\linewidth}{!}{
    \begin{subfigure}[b]{1.0\linewidth}
        \includegraphics[width=\linewidth]{supmat/figs/poses/pigan/p_2.pdf}
    \end{subfigure}
    \begin{subfigure}[b]{1.0\linewidth}
        \includegraphics[width=\linewidth]{supmat/figs/poses/pigan/p_3.pdf}
    \end{subfigure}
    }
    \resizebox{1.0\linewidth}{!}{
    \begin{subfigure}[b]{1.0\linewidth}
        \includegraphics[width=\linewidth]{supmat/figs/poses/pigan/p_4.pdf}
    \end{subfigure}
    \begin{subfigure}[b]{1.0\linewidth}
        \includegraphics[width=\linewidth]{supmat/figs/poses/pigan/p_5.pdf}
    \end{subfigure}
    }
    \caption{
    Images generated by the original Pi-GAN~\cite{pigan} with different \emph{poses}.}
    \label{Fig:poses_pigan}
\end{figure*}

\newpage

\begin{figure*}[t!]
    \centering
    \resizebox{1.0\linewidth}{!}{
    \begin{subfigure}[b]{1.0\linewidth}
        \includegraphics[width=\linewidth]{supmat/figs/poses/cgof/c_0.pdf}
    \end{subfigure}
    \begin{subfigure}[b]{1.0\linewidth}
        \includegraphics[width=\linewidth]{supmat/figs/poses/cgof/c_1.pdf}
    \end{subfigure}
    }
    \resizebox{1.0\linewidth}{!}{
    \begin{subfigure}[b]{1.0\linewidth}
        \includegraphics[width=\linewidth]{supmat/figs/poses/cgof/c_2.pdf}
    \end{subfigure}
    \begin{subfigure}[b]{1.0\linewidth}
        \includegraphics[width=\linewidth]{supmat/figs/poses/cgof/c_3.pdf}
    \end{subfigure}
    }
    \resizebox{1.0\linewidth}{!}{
    \begin{subfigure}[b]{1.0\linewidth}
        \includegraphics[width=\linewidth]{supmat/figs/poses/cgof/c_4.pdf}
    \end{subfigure}
    \begin{subfigure}[b]{1.0\linewidth}
        \includegraphics[width=\linewidth]{supmat/figs/poses/cgof/c_5.pdf}
    \end{subfigure}
    }
    \caption{
    Images generated by our proposed cGOF with different \emph{poses}.}
    \label{Fig:poses_cgof}
\end{figure*}

\newpage

\begin{figure*}[t!]
    \centering
    \resizebox{1.0\linewidth}{!}{
        \includegraphics[width=\linewidth]{supmat/figs/exps/gancontrol/gan_control_exp_red.pdf}
    }
    \caption{Images generated by \ganctrlc with different \emph{expressions}.
    Each row is generated with the same parameters except the expression code, and each column shares the same expression code.
    Red boxes highlight examples where \ganctrl produces severe inconsistencies in the identity and background when only the expression is supposed to change.
    Moreover, we notice the ``smiling'' attribute tends to strongly correlate with the ``female'' and ``long-hair'' attributes.
    }
    \label{Fig:exps_gancontrol}
\end{figure*}

\begin{figure*}[t!]
    \centering
    \resizebox{1.0\linewidth}{!}{
        \includegraphics[width=\linewidth]{supmat/figs/exps/disco/discofacegan_exp_blue1.pdf}
    }
    \caption{Images generated by \discoc with different \emph{expressions}.
    Each row is generated with the same parameters except the expression code, and each column shares the same expression code.
    Blue boxes highlight some examples where \disco fails to produce consistent expressions among different instances.
    }
    \label{Fig:exps_disco}
\end{figure*}

\begin{figure*}[t!]
    \centering
    \resizebox{1.0\linewidth}{!}{
        \includegraphics[width=\linewidth]{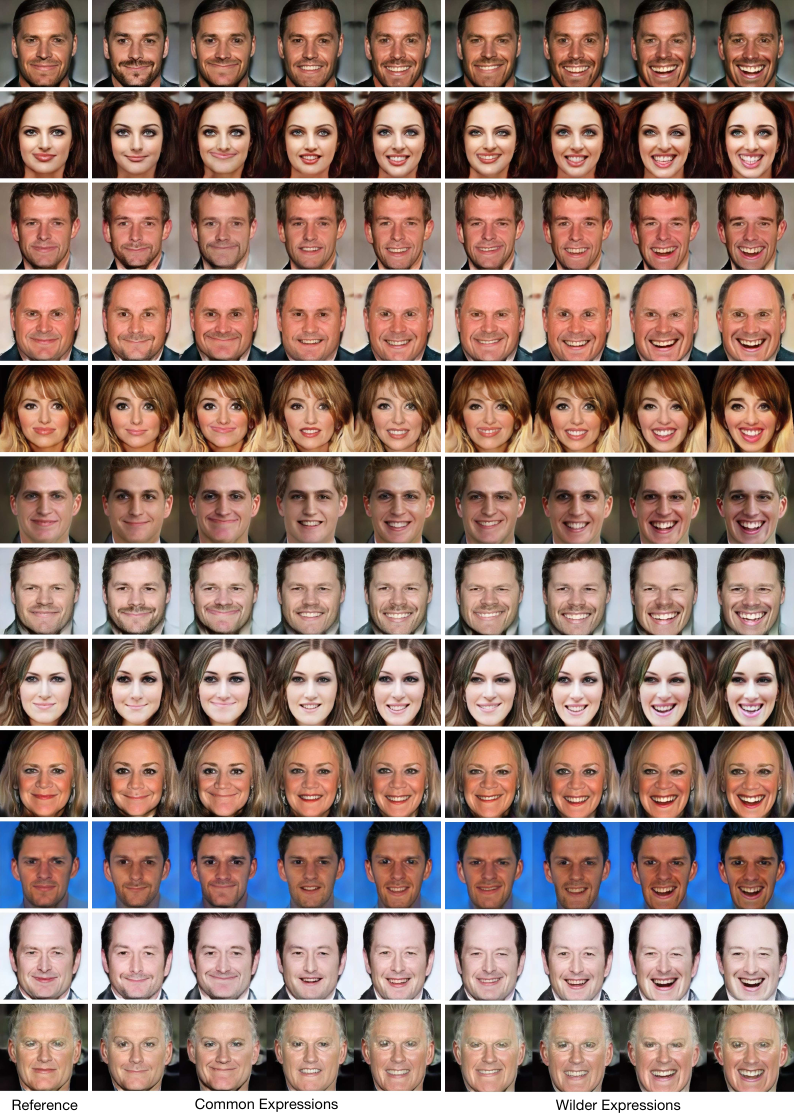}
    }
    \caption{Images generated by our proposed cGOF with different \emph{expressions}.
    Our model generates photo-realistic face images with highly consistent, precise expression control.}
    \label{Fig:exps_cgof}
\end{figure*}

\begin{figure*}[t!]
    \centering
    \resizebox{1.0\linewidth}{!}{
        \includegraphics[width=\linewidth]{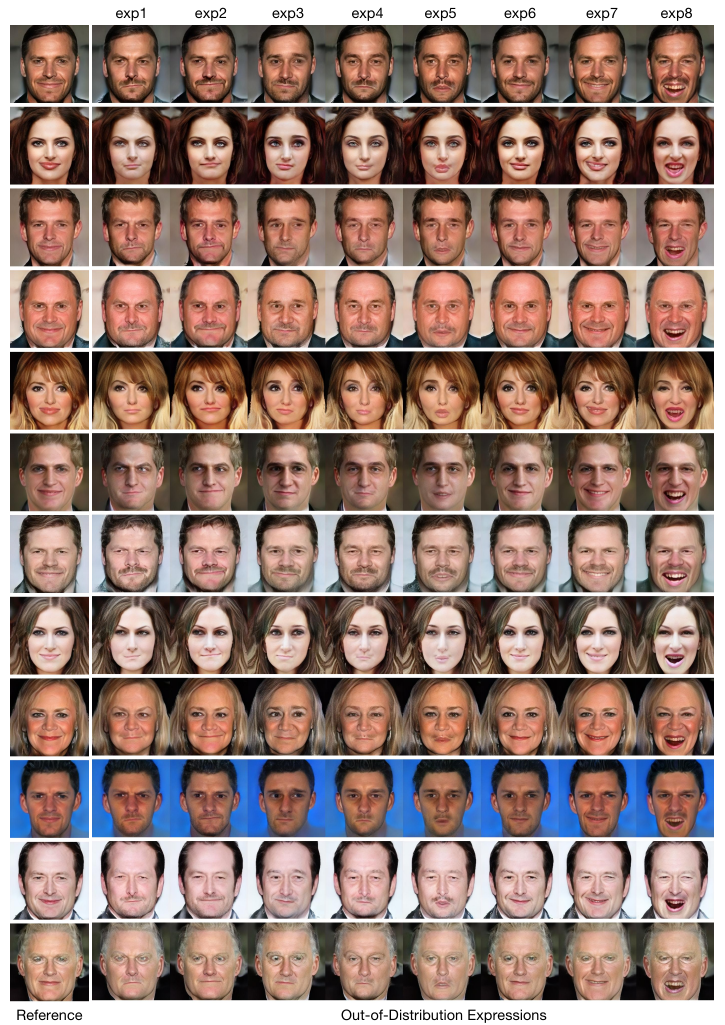}
    }
    \caption{Images generated by our proposed cGOF with \emph{out-of-distribution} \emph{expressions}.
    Our method is capable of synthesizing unseen expressions like raising eyebrow, pouting, curling lips, smirking \etc.}
    \label{Fig:exps_ood_cgof}
\end{figure*}
