# Supplementary material for: CGOF++: Controllable 3D Face Synthesis with Conditional Generative Occupancy Fields
Source: arXiv:2211.13251 source file (2023-10-29)
Supplement: Supplementary file 3 [file cgof_ood.tex]

\begin{figure*}[t!]
    \centering
    \resizebox{1.0\linewidth}{!}{
        \includegraphics[width=\linewidth]{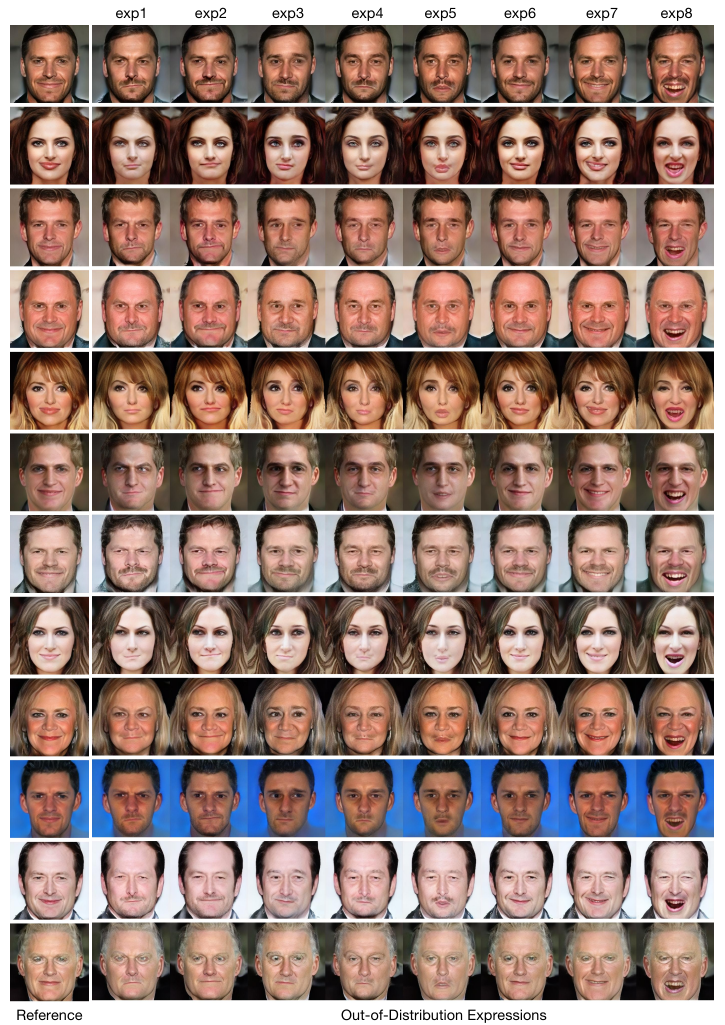}
    }
    \caption{Images generated by our proposed cGOF with \emph{out-of-distribution} \emph{expressions}.
    Our method is capable of synthesizing unseen expressions like raising eyebrow, pouting, curling lips, smirking \etc.}
    \label{Fig:exps_ood_cgof}
\end{figure*}
