# Supplementary material for: CGOF++: Controllable 3D Face Synthesis with Conditional Generative Occupancy Fields
Source: arXiv:2211.13251 source file (2023-10-29)
Supplement: Supplementary file 4 [file disco.tex]

\begin{figure*}[t!]
    \centering
    \resizebox{1.0\linewidth}{!}{
        \includegraphics[width=\linewidth]{supmat/figs/exps/disco/discofacegan_exp_blue1.pdf}
    }
    \caption{Images generated by \discoc with different \emph{expressions}.
    Each row is generated with the same parameters except the expression code, and each column shares the same expression code.
    Blue boxes highlight some examples where \disco fails to produce consistent expressions among different instances.
    }
    \label{Fig:exps_disco}
\end{figure*}
