# Supplementary material for: CGOF++: Controllable 3D Face Synthesis with Conditional Generative Occupancy Fields
Source: arXiv:2211.13251 source file (2023-10-29)
Supplement: Supplementary file 5 [file gancontrol.tex]

\begin{figure*}[t!]
    \centering
    \resizebox{1.0\linewidth}{!}{
        \includegraphics[width=\linewidth]{supmat/figs/exps/gancontrol/gan_control_exp_red.pdf}
    }
    \caption{Images generated by \ganctrlc with different \emph{expressions}.
    Each row is generated with the same parameters except the expression code, and each column shares the same expression code.
    Red boxes highlight examples where \ganctrl produces severe inconsistencies in the identity and background when only the expression is supposed to change.
    Moreover, we notice the ``smiling'' attribute tends to strongly correlate with the ``female'' and ``long-hair'' attributes.
    }
    \label{Fig:exps_gancontrol}
\end{figure*}
