# Supplementary material for: CGOF++: Controllable 3D Face Synthesis with Conditional Generative Occupancy Fields
Source: arXiv:2211.13251 source file (2023-10-29)
Supplement: Supplementary file 7 [file disco.tex]

\begin{figure*}[t!]
    \centering
    \resizebox{1.0\linewidth}{!}{
    \begin{subfigure}[b]{1.0\linewidth}
        \includegraphics[width=\linewidth]{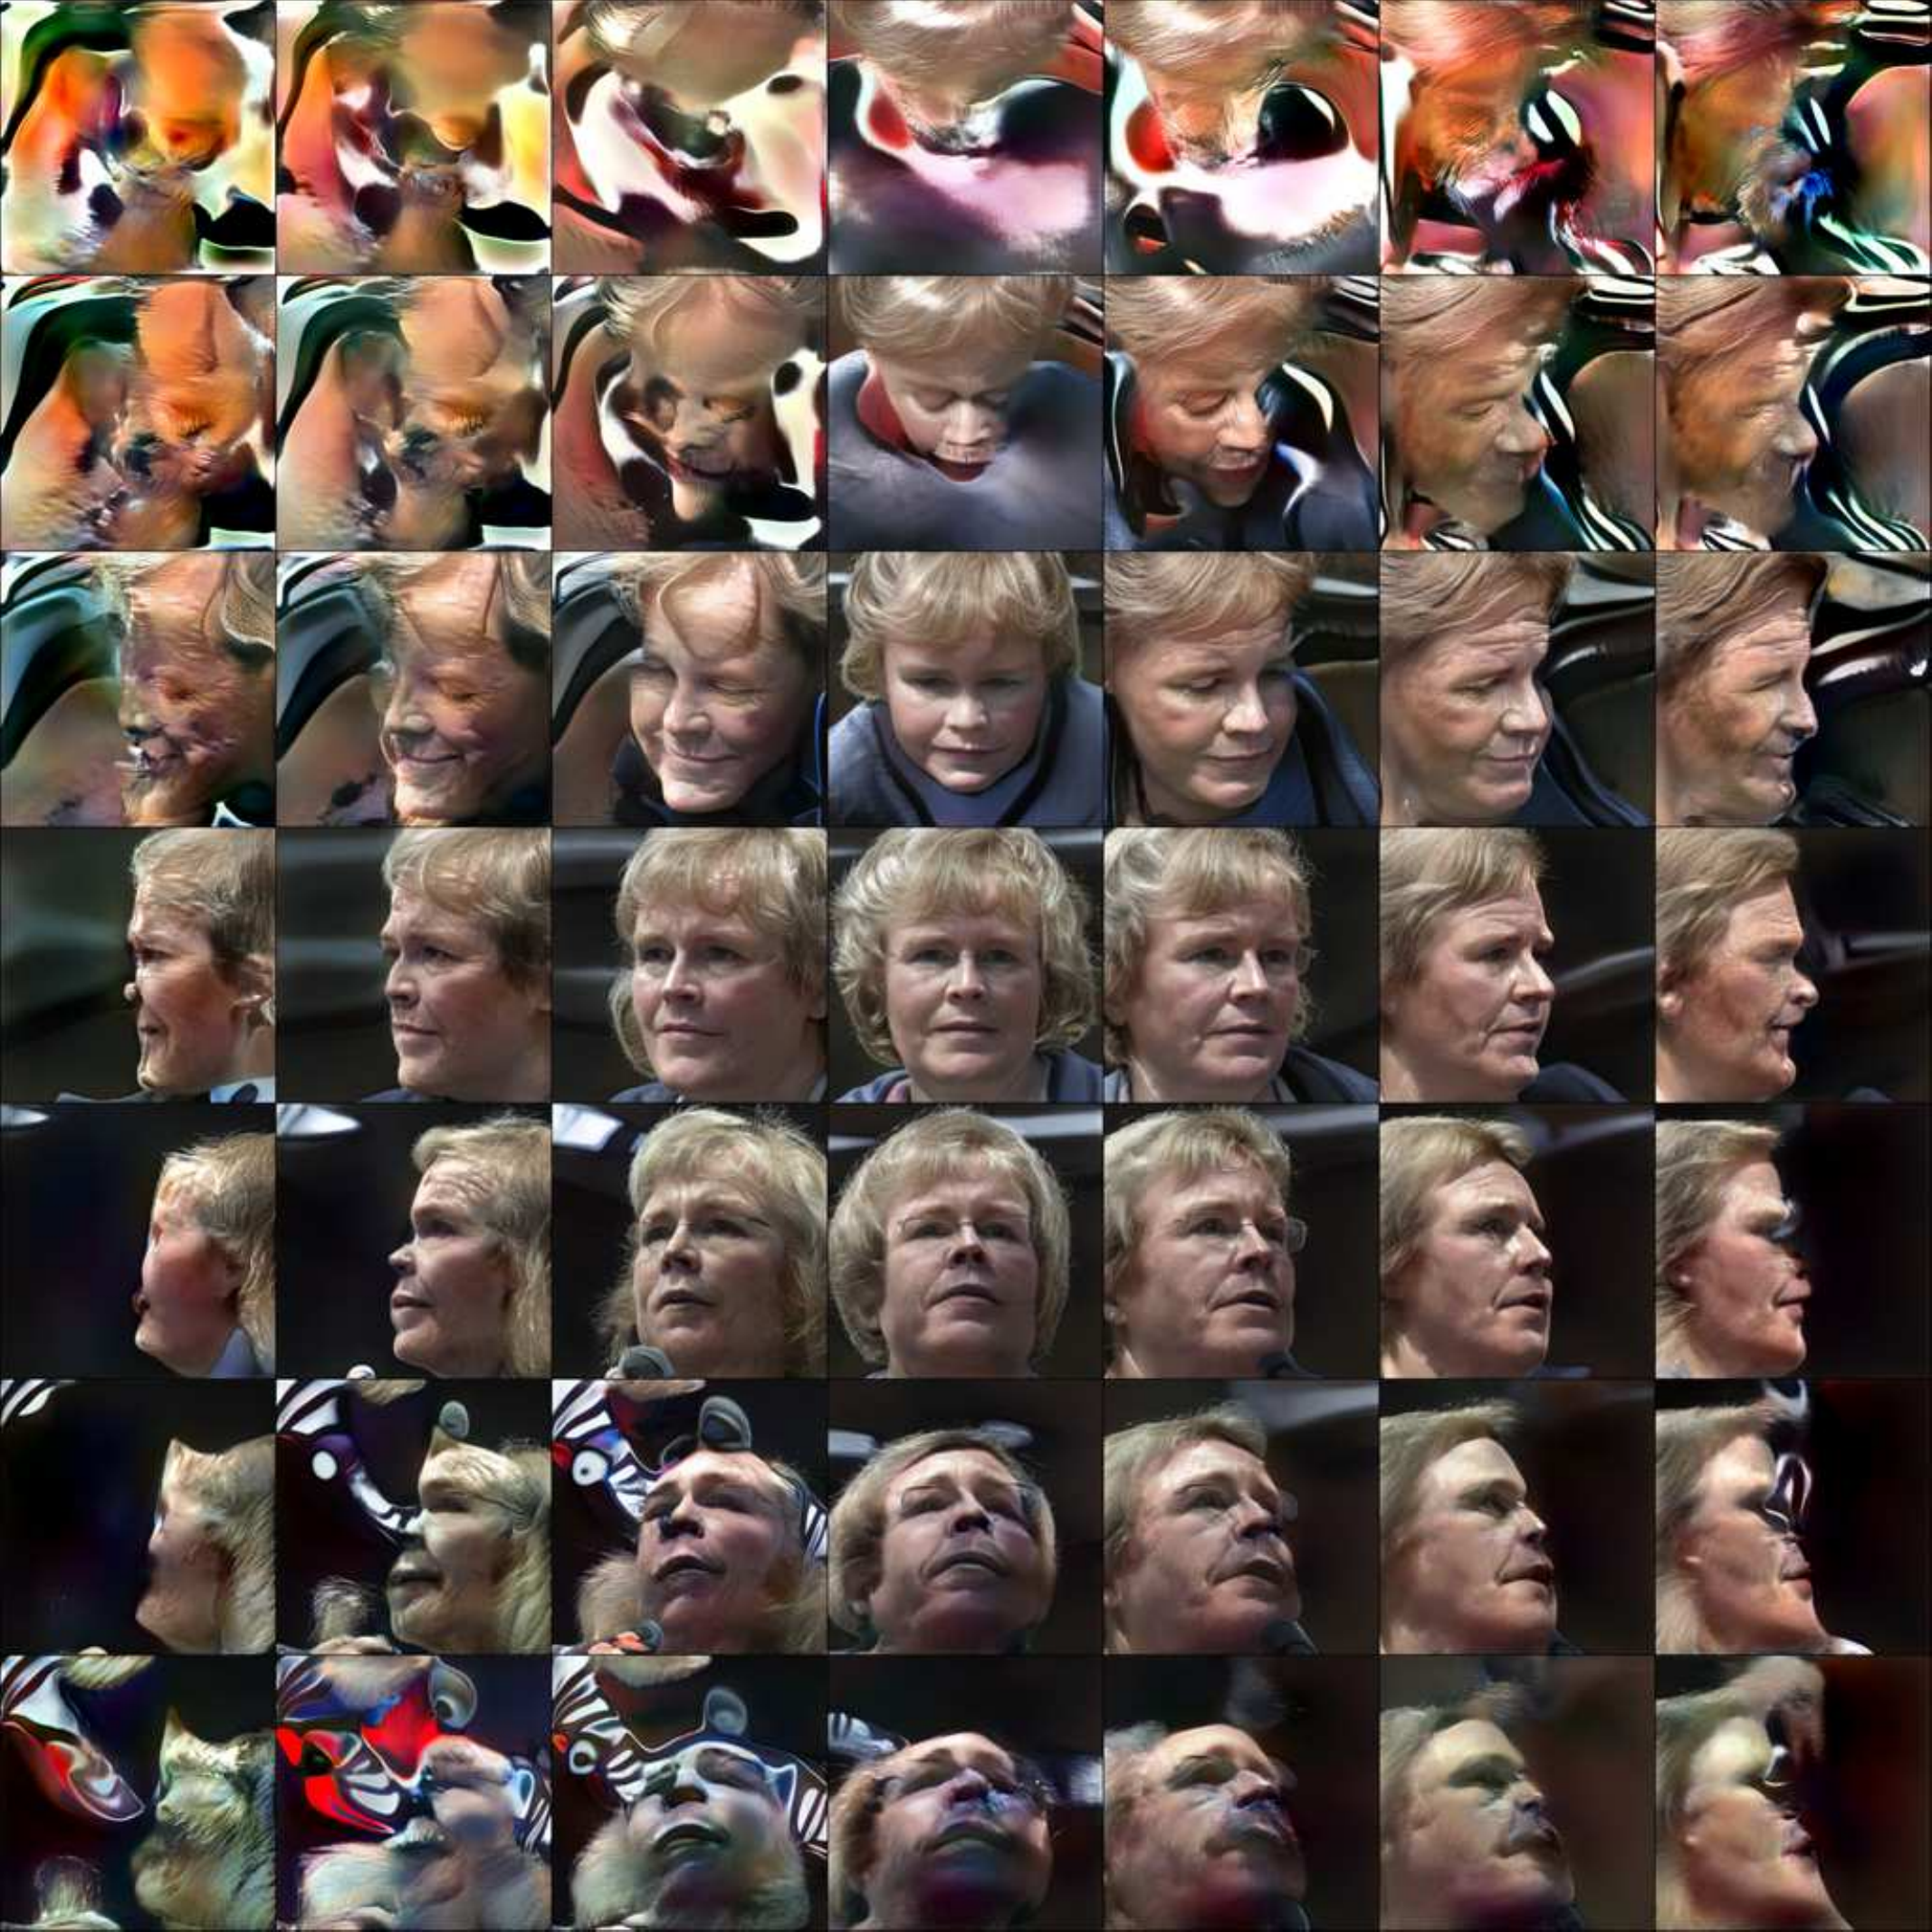}
    \end{subfigure}
    \begin{subfigure}[b]{1.0\linewidth}
        \includegraphics[width=\linewidth]{supmat/figs/poses/disco/d_1_1024.pdf}
    \end{subfigure}
    }
    \resizebox{1.0\linewidth}{!}{
    \begin{subfigure}[b]{1.0\linewidth}
        \includegraphics[width=\linewidth]{supmat/figs/poses/disco/d_2_1024.pdf}
    \end{subfigure}
    \begin{subfigure}[b]{1.0\linewidth}
        \includegraphics[width=\linewidth]{supmat/figs/poses/disco/d_3_1024.pdf}
    \end{subfigure}
    }
    \resizebox{1.0\linewidth}{!}{
    \begin{subfigure}[b]{1.0\linewidth}
        \includegraphics[width=\linewidth]{supmat/figs/poses/disco/d_4_1024.pdf}
    \end{subfigure}
    \begin{subfigure}[b]{1.0\linewidth}
        \includegraphics[width=\linewidth]{supmat/figs/poses/disco/d_5_1024.pdf}
    \end{subfigure}
    }
    \caption{Images generated by DiscoFaceGAN~\cite{deng2020disentangled} with different \emph{poses}.}
    \label{Fig:poses_disco}
\end{figure*}
