# Supplementary material for: CGOF++: Controllable 3D Face Synthesis with Conditional Generative Occupancy Fields
Source: arXiv:2211.13251 source file (2023-10-29)
Supplement: Supplementary file 10 [file pigan.tex]

\begin{figure*}[t!]
    \centering
    \resizebox{1.0\linewidth}{!}{
    \begin{subfigure}[b]{1.0\linewidth}
        \includegraphics[width=\linewidth]{supmat/figs/poses/pigan/p_0.pdf}
    \end{subfigure}
    \begin{subfigure}[b]{1.0\linewidth}
        \includegraphics[width=\linewidth]{supmat/figs/poses/pigan/p_1.pdf}
    \end{subfigure}
    }
    \resizebox{1.0\linewidth}{!}{
    \begin{subfigure}[b]{1.0\linewidth}
        \includegraphics[width=\linewidth]{supmat/figs/poses/pigan/p_2.pdf}
    \end{subfigure}
    \begin{subfigure}[b]{1.0\linewidth}
        \includegraphics[width=\linewidth]{supmat/figs/poses/pigan/p_3.pdf}
    \end{subfigure}
    }
    \resizebox{1.0\linewidth}{!}{
    \begin{subfigure}[b]{1.0\linewidth}
        \includegraphics[width=\linewidth]{supmat/figs/poses/pigan/p_4.pdf}
    \end{subfigure}
    \begin{subfigure}[b]{1.0\linewidth}
        \includegraphics[width=\linewidth]{supmat/figs/poses/pigan/p_5.pdf}
    \end{subfigure}
    }
    \caption{
    Images generated by the original Pi-GAN~\cite{pigan} with different \emph{poses}.}
    \label{Fig:poses_pigan}
\end{figure*}
